# Supplementary material for: Automatic Synthesis of Random Generators for Numerically Constrained Algebraic Recursive Types
Source: arXiv:2208.12747 source file (2022-08-26)
Supplement: Supplementary file 1 [file appendice.tex]

\section{BST: Constructive Approach is not Uniform\label{bstnonuniform}}
Inserting a node $n$ consists in recursively inserting $n$ to the
left subtree if its key is less than that of the root or to the
right subtree otherwise. New keys are always inserted in leaf
position. Figure~\ref{fig:nonu} shows that building trees by
generating a random sequence of insertions favours the apparition
on some values rather than others, namely the tree obtained in
figure~\ref{fig:morefrequent}.

\begin{figure}[h]
    \centering
    \subfloat[\centering Insertion order: 1,2,3]{
    \begin{forest}
for tree={
    grow=south,
    circle, draw, minimum size=3ex, inner sep=1pt,
    s sep=7mm
        }
    [1[,no edge, draw=none][2 [,no edge, draw=none] [3]]]
\end{forest}}%
    \qquad
    \centering
    \subfloat[\centering Insertion order: 1,3,2]{
    \begin{forest}
    for tree={
    grow=south,
    circle, draw, minimum size=3ex, inner sep=1pt,
    s sep=7mm
    }
    [1 [,no edge, draw=none] [3 [2] [,no edge, draw=none]]]
\end{forest}}%
    \qquad
    \centering
    \subfloat[\centering Insertion order: 2,1,3 \& 2,3,1\label{fig:morefrequent}]{
\begin{forest}
for tree={
    grow=south,
    circle, draw, minimum size=3ex, inner sep=1pt,
    s sep=7mm
        }
        [2 [1] [3]]
\end{forest}}%
    \qquad
    \centering
    \subfloat[\centering Insertion order: 3,2,1]{
\begin{forest}
for tree={
    grow=south,
    circle, draw, minimum size=3ex, inner sep=1pt,
    s sep=7mm
        }
    [3 [2 [1][,no edge, draw=none]][,no edge, draw=none]]
\end{forest}}%
    \qquad
    \centering
    \subfloat[\centering Insertion order: 3,1,2]{
\begin{forest}
for tree={
    grow=south,
    circle, draw, minimum size=3ex, inner sep=1pt,
    s sep=7mm
        }
    [3 [1[,no edge, draw=none][2]][,no edge, draw=none]]
\end{forest}}
\caption{All possible BST of size three with values: $\{1,2,3\}$}
\label{fig:nonu}
\end{figure}

\section{Generated code for BST\label{gencodebst}}
\begin{figure}[h]
\begin{lstlisting}{ocaml}
type bst = Node of bst * (int[@collect]) * bst | Leaf
[@@satisfying increasing]

let rec insert (x : int) (bt : bst) : bst =
  match bt with
  | Leaf -> Node (Leaf, x, Leaf)
  | Node (l, x', r) ->
      if x < x' then Node(insert x l, x', r) else Node(l, x', insert x r)
\end{lstlisting}
\caption{An OCaml program that manipulates binary search trees\label{fig:bst}}
\end{figure}

\begin{figure}[h]
\begin{lstlisting}{ocaml}
let () =
  let generator rs =
    let x1 = QCheck.Gen.int rs in
    let x2 =
      let rec of_arbogen_bst arbg queue rs =
        Arbogen.(
          match arbg with
          | Tree.Label ("bst", [Tuple []; child]) -> (
            match child with
            | Tree.Label ("Node", [x1; x2; x3]) ->
                let x1, x2, x3 =
                  let x1 = of_arbogen_bst x1 queue rs in
                  let x2 = Testify_runtime.Arbg.to_int x2 queue rs in
                  let x3 = of_arbogen_bst x3 queue rs in
                  (x1, x2, x3)
                in
                Node (x1, x2, x3)
            | Tree.Label ("Leaf", []) -> Leaf
            | x -> failwith "Ill-formed arbogen tree" )
          | x -> failwith "Ill-formed arbogen tree")
      in
      let wg =
        let open Arbogen.Boltzmann.WeightedGrammar in
        { names= [|"bst"; "Node"; "Leaf"; "@collect"|]
        ; rules=
            [| Union
                 [ (0.499977638879, Product [Z 1; Ref 1])
                 ; (0.500022361122, Product [Z 1; Ref 2]) ]
             ; Product [Ref 0; Ref 3; Ref 0]
             ; Z 0
             ; Z 0 |] }
      in
      let tree = Testify_runtime.Arbg.generate wg "bst" rs in
      let nb_collect = Testify_runtime.Arbg.count_collect tree in
      let queue =
        (fun n -> [|Testify_runtime.Sicstus.increasing_list n|]) nb_collect
      in
      of_arbogen_bst tree queue rs
    in
    let rec print_bst = function
      | Node (x1, x2, x3) ->
          "Node"
          ^ ( "("
            ^ (print_bst x1 ^ ", " ^ string_of_int x2)
            ^ ", " ^ print_bst x3 )
          ^ ")"
      | Leaf -> "Leaf"
    in
    let x3 = insert x1 x2 in
    ( x3
    , (("(insert " ^ string_of_int x1 ^ " " ^ print_bst x2) ^ ")")
      ^ " = " ^ print_bst x3 )
  in
  Testify_runtime.(
    add_fun 0x2710 "insert"
      "File \"examples/recursive/bst.ml\", lines 4-8, characters 0-75"
      (opt_print snd) (opt_gen generator)
      (sat_output
         (let open Operators in
         let rec collect_bst n = function
           | Node (x1, x2, x3) ->
               (fun n (x1, x2, x3) ->
                 List.flatten
                   [ collect_bst n x1
                   ; (if n = 0 then Collect.int n else fun x -> []) x2
                   ; collect_bst n x3 ] )
                 n (x1, x2, x3)
           | Leaf -> []
         in
         fun x -> increasing ((collect_bst 0) x)) ))

let () = Testify_runtime.run_test ()
\end{lstlisting}
\caption{Test generated for the function insert\label{fig:bst-generated-code}}
\end{figure}

\section{Type definitions for the Types used in Section~\ref{sec:bench}\label{app:types}}
\begin{figure}[h]
\begin{lstlisting}{ocaml}
type increasing_list =
  | Nil 
  | Cons of ((int)[@collect ]) * increasing_list 
[@@satisfying increasing]

type assoc_list =
  | Nil 
  | Cons of ((int)[@collect ]) * int * assoc_list
[@@satisfying alldiff]

type bicollect = 
  | Empty
  | Cons of (int[@collect 1]) * (int[@collect 2]) * bicollect
[@@satisfying fun x -> increasing x 1 && increasing x 2]

type binary_tree = 
  | Node of binary_tree * (int[@collect]) * binary_tree
  | Leaf
[@@satisfying increasing]

type map = 
  | Node of map * (int[@collect]) * int * map
  | Leaf
[@@satisfying increasing]

type quad_tree_x =
  | LeafX
  | NodeX of
      (int[@collect 1])
      * quad_tree_y
      * quad_tree_y
      * (int[@collect 2])
[@@satisfying fun x -> increasing x 1 && increasing x 2]
and quad_tree_y =
  | LeafY
  | NodeY of
      (int[@collect 3])
      * quad_tree_x
      * quad_tree_x
      * (int[@collect 4])
[@@satisfying fun x -> increasing x 3 && increasing x 4]
\end{lstlisting}
\caption{Constrained Types Used in Experiments }
\end{figure}
